# Supplementary material for: Online Photometric Calibration of Automatic Gain Thermal Infrared Cameras
Source: arXiv:2012.14292 source file (2021-01-11)
Supplement: Supplementary file 1 [file appendix.tex]

\appendix
	
	\section{Appendix: Dataset Details}
	We discuss in details the dataset used for the experiments and attempt to convey the associated challenges. We use two types of datasets:
	\begin{enumerate}
		\item Publicly-available Dataset (All-Day Visual Place Recognition: Benchmark Dataset and Baselines\footnote{Source \href{https://sites.google.com/site/alldaydataset/dataset-info}{https://sites.google.com/site/alldaydataset/dataset-info}}) from Korean Advanced Institute of Science \& Technology (KAIST). The thermal images were captured using a FLIR A35 SC camera atop a moving vehicle. \autoref{fig:kaist-dataset} shows a few images from the KAIST dataset.
		\item A custom dataset we collected using a FLIR A65 camera mounted on a Micro-Aerial Vehicle (MAV). The camera is mounted at various angles on the MAV, and an angle of $90^\circ$ means that the camera is downward facing. \autoref{fig:A65_A-dataset}, \autoref{fig:A65_C-dataset} \& \autoref{fig:A65_D-dataset} shows a few images with different camera angles.
	\end{enumerate}
	\begin{figure*}[h!]
		\centering
		\subfloat{\includegraphics[width=0.16\textwidth]{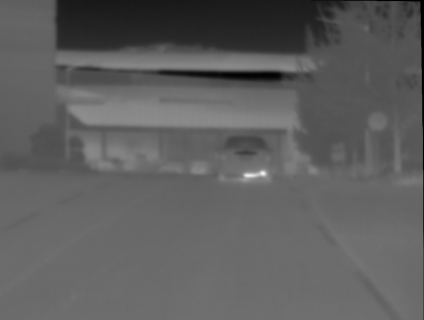}}
		\hfill
		\subfloat{\includegraphics[width=0.16\textwidth]{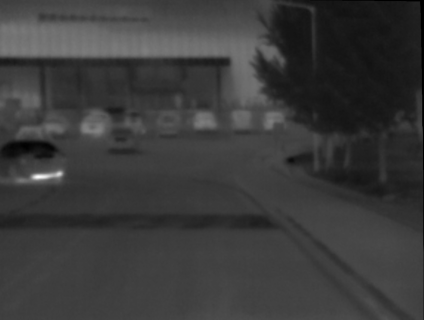}}
		\hfill
		\subfloat{\includegraphics[width=0.16\textwidth]{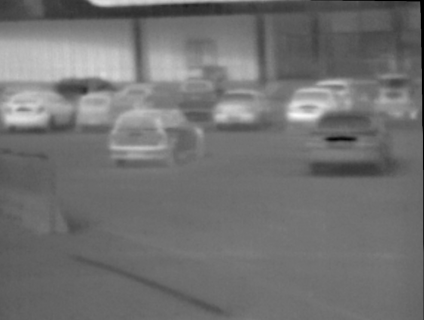}}
		\hfill
		\subfloat{\includegraphics[width=0.16\textwidth]{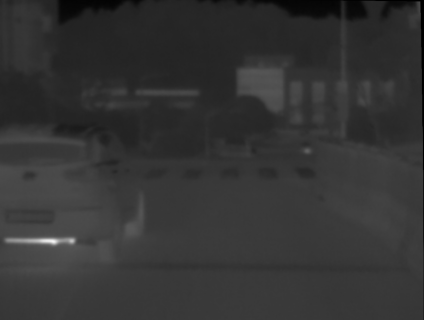}}
		\hfill
		\subfloat{\includegraphics[width=0.16\textwidth]{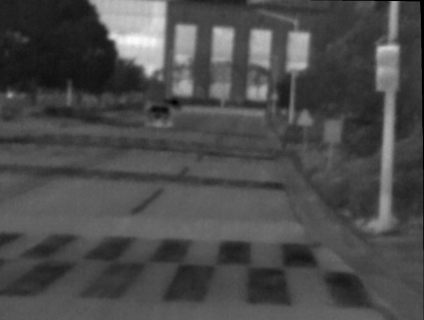}}
		\hfill
		\subfloat{\includegraphics[width=0.16\textwidth]{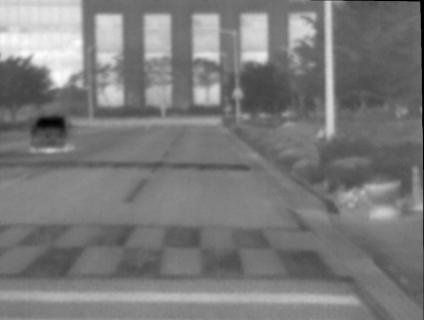}}
		\caption{\small Sample Images from Dataset KAIST AM02.}
		\label{fig:kaist-dataset}
	\end{figure*}
	\begin{figure*}[h!]
		\centering
		\subfloat{\includegraphics[width=0.16\textwidth]{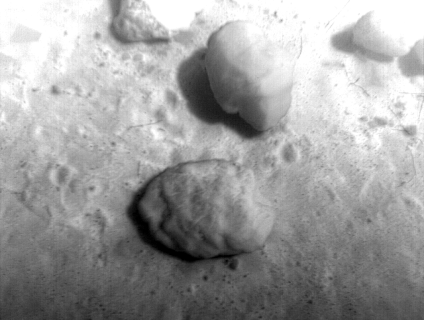}}
		\hfill
		\subfloat{\includegraphics[width=0.16\textwidth]{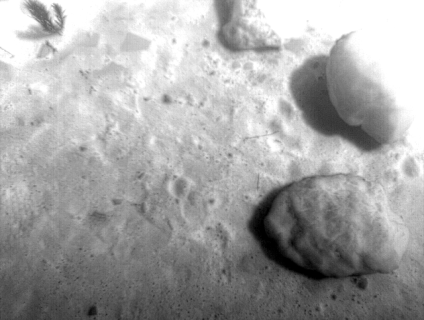}}
		\hfill
		\subfloat{\includegraphics[width=0.16\textwidth]{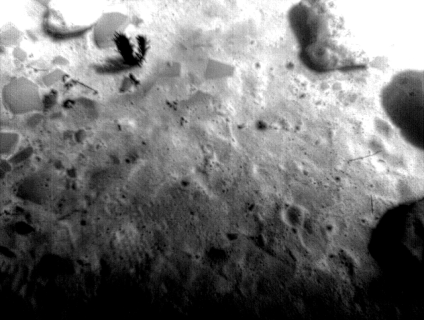}}
		\hfill
		\subfloat{\includegraphics[width=0.16\textwidth]{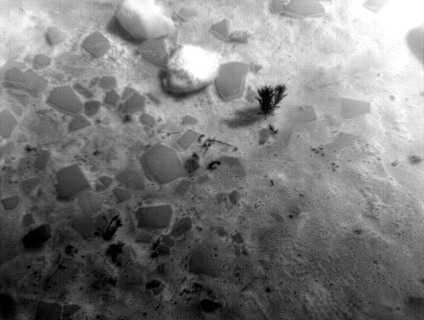}}
		\hfill
		\subfloat{\includegraphics[width=0.16\textwidth]{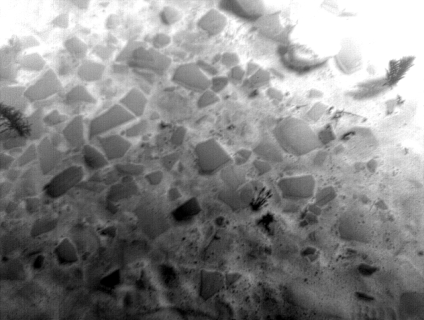}}
		\hfill
		\subfloat{\includegraphics[width=0.16\textwidth]{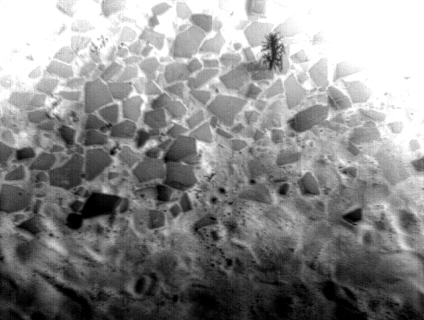}}
		\caption{\small Sample Images from Dataset MAV\_A. Camera at $85^\circ$}
		\label{fig:A65_A-dataset}
	\end{figure*}
	\begin{figure*}[h!]
		\centering
		\subfloat{\includegraphics[width=0.16\textwidth]{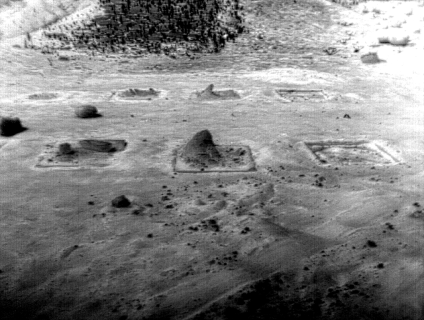}}
		\hfill
		\subfloat{\includegraphics[width=0.16\textwidth]{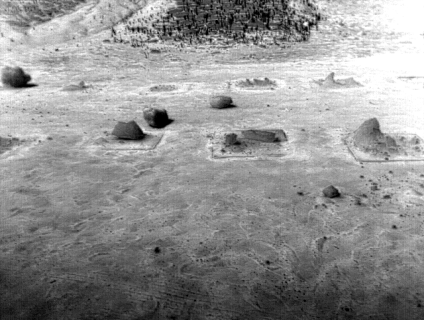}}
		\hfill
		\subfloat{\includegraphics[width=0.16\textwidth]{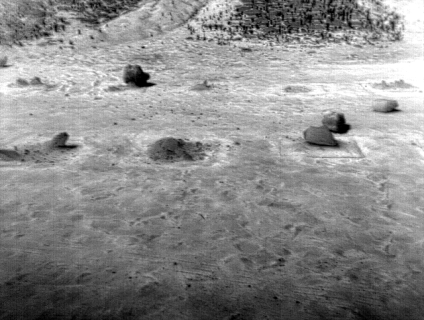}}
		\hfill
		\subfloat{\includegraphics[width=0.16\textwidth]{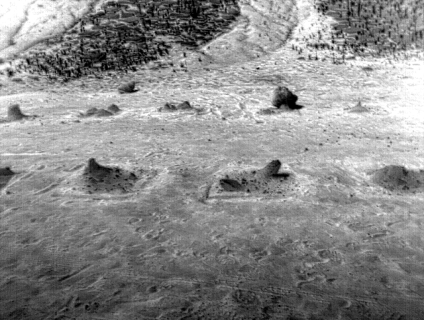}}
		\hfill
		\subfloat{\includegraphics[width=0.16\textwidth]{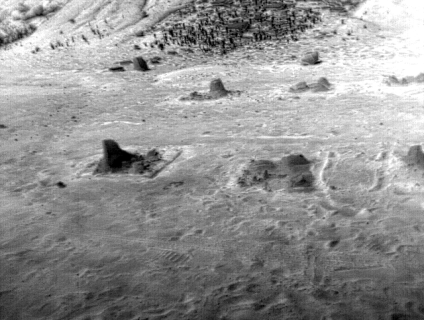}}
		\hfill
		\subfloat{\includegraphics[width=0.16\textwidth]{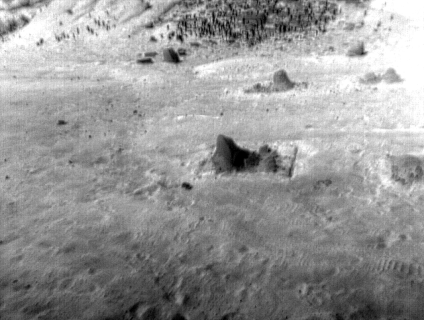}}
		\caption{\small  Sample Images from Dataset MAV\_B. Camera at $35^\circ$}
		\label{fig:A65_C-dataset}
	\end{figure*}
	\begin{figure*}[h!]
		\centering
		\subfloat{\includegraphics[width=0.16\textwidth]{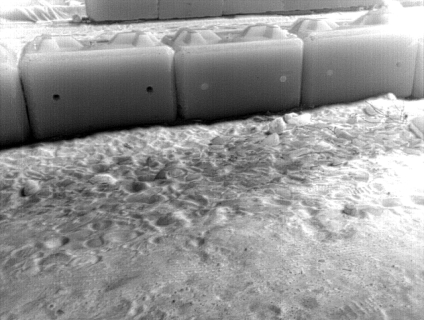}}
		\hfill
		\subfloat{\includegraphics[width=0.16\textwidth]{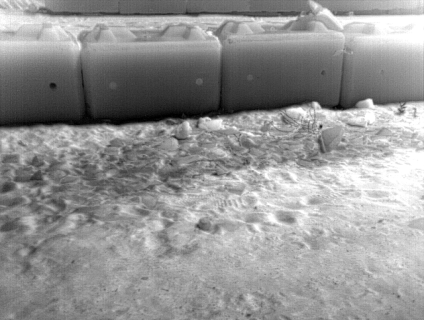}}
		\hfill
		\subfloat{\includegraphics[width=0.16\textwidth]{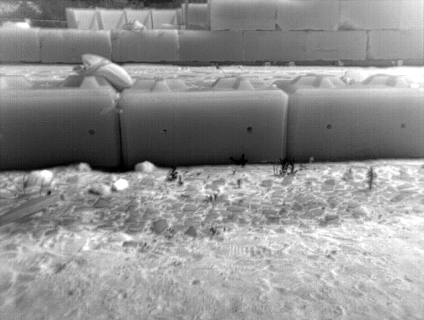}}
		\hfill
		\subfloat{\includegraphics[width=0.16\textwidth]{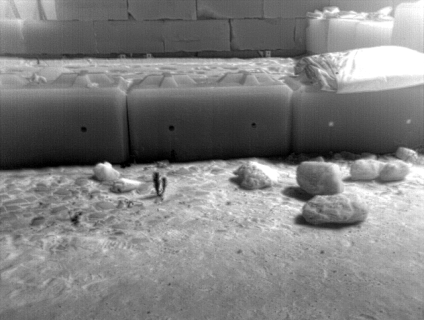}}
		\hfill
		\subfloat{\includegraphics[width=0.16\textwidth]{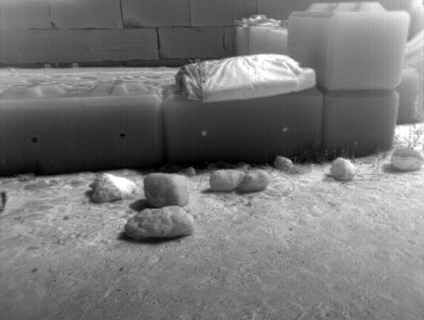}}
		\hfill
		\subfloat{\includegraphics[width=0.16\textwidth]{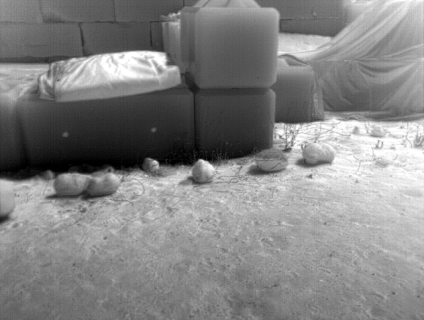}}
		\caption{\small  Sample Images from Dataset MAV\_C. Camera at $10^\circ$}
		\label{fig:A65_D-dataset}
	\end{figure*}
	
	We can clearly notice that the KAIST dataset exhibits wide temporal variation, while the MAV dataset exhibits high spatial variations. The corners (especially the top-right corner) in the MAV images seem to be ``over-exposed''.
	
	\section{Appendix: Experiment Details}
	\subsubsection{Benefits to Feature Tracking:}
	Here we elaborate on the computation of Pearson correlation coefficient $\rho$ and how does it measure the performance of our proposed method. Refer to the \autoref{fig:klt-video-image}, frame ($t-1$) shows the features initialized by KLT. We can clearly observe that there exists a temporal variation between the two frames (\textbf{Left} $t-1$ and \textbf{Right} $t$). The calibrated version of $t$ (\textbf{Mid}) attempts to remove this photometric error and make world points appear similar to how they appear in $t-1$. In this example, we can clearly observe that the number of points tracked to the uncalibrated version is far less than that to the calibrated version. Next we measure the photometric error based on the estimated temporal parameters. Recall that $P'_t$ contains $P'_{1,t-1} = \{{}^1a_{t-1}, {}^1b_{t-1}\}$ and $P'_{1,t} = \{{}^1a_{t}, {}^1b_{t}\}$. We compute ${}^1c_{t-1} = e^{{}^1a_{t-1}} + {}^1b_{t-1}$ and ${}^1c_{t} = e^{{}^1a_{t}} + {}^1b_{t}$. Also recall that, $c_t$ \& $b_t$ are estimates of $I'_{t,\text{max}}$ \& $I'_{t,\text{min}}$ respectively. The photometric difference is thus $\delta = \sqrt{ ({}^1c_{t-1}-{}^1c_{t})^2  + ({}^1b_{t-1}-{}^1b_{t})^2}$. We filter pairs of frames based on various thresholds on $\delta$. \autoref{fig:klt-points} shows the scatter plot for three different thresholds between normalized difference $\hat{g}$ and photometric error $\delta$. The experiments quantify the Pearson correlation coefficient between $\hat{g}$ and $\delta$.
	\begin{figure}[h!]
		\centering
		\subfloat{\includegraphics[width=\linewidth]{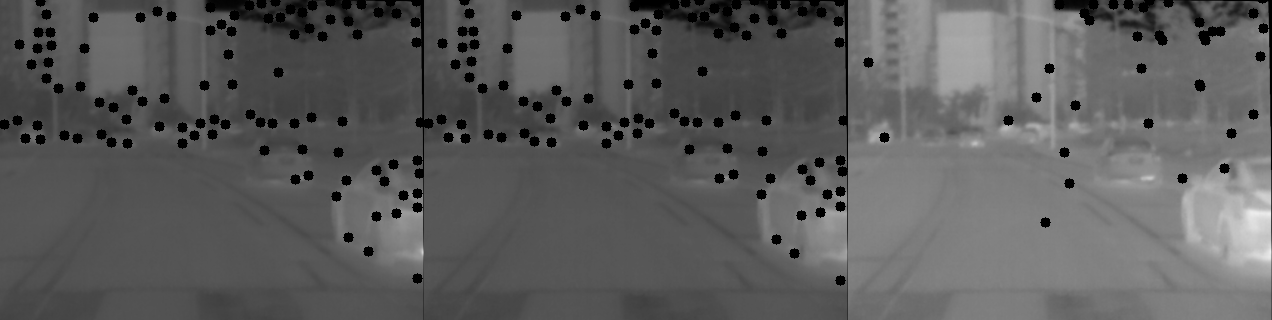}}
		\caption{\small A qualitative result of the KLT feature tracking with and without photometric calibration. \textbf{Left:} Image at frame $t-1$. \textbf{Center:} Calibrated version of frame $t$. \textbf{Right:} Uncalibrated version of frame $t$.} 
		\label{fig:klt-video-image}
	\end{figure}
	\begin{figure}[h!]
		\centering
		\subfloat{\includegraphics[width=0.32\linewidth]{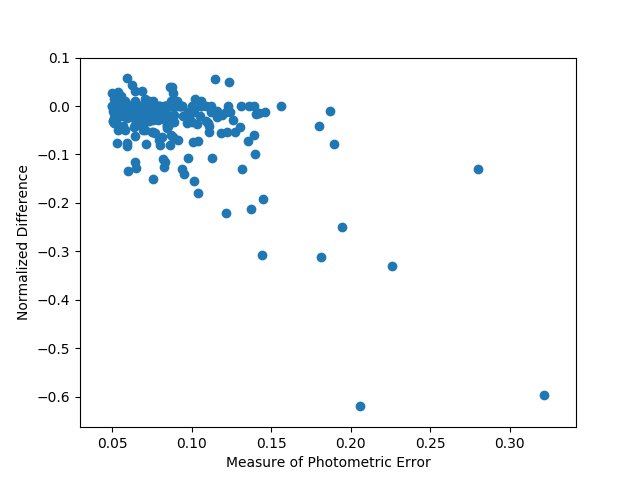}}\hfill
		\subfloat{\includegraphics[width=0.32\linewidth]{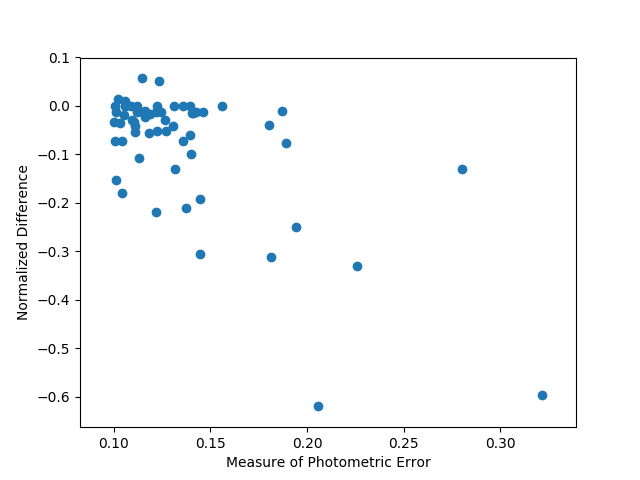}}\hfill
		\subfloat{\includegraphics[width=0.32\linewidth]{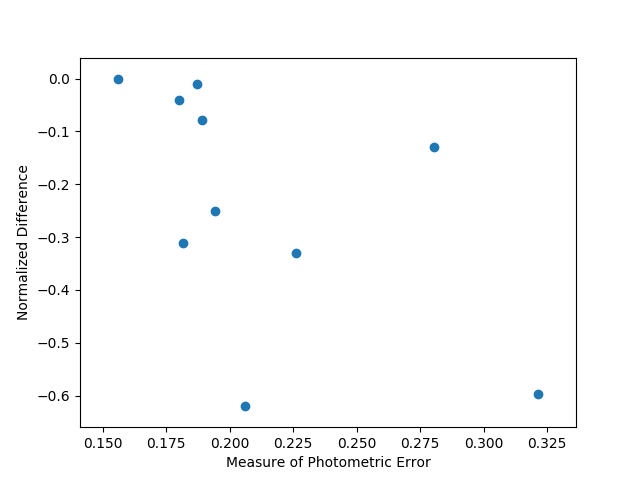}}
		\caption{\small \textbf{Left:} $\delta \geq 0.05$, \textbf{Center:} $\delta \geq 0.1$, \textbf{Right:} $\delta \geq 0.15$} 
		\label{fig:klt-points}
	\end{figure}
	
	\autoref{fig:t_v_corr} plots the Pearson correlation coefficient as a function of various thresholds. The coefficient is less negative for lower thresholds due to noise, whereas the coefficient is more negative for higher thresholds. However since less number of frame pairs are used to estimate correlation at higher thresholds, thus the estimate is more uncertain. We therefore, choose the three thresholds to show the two extreemes ($\delta \geq 0.05$ \& $\delta \geq 0.15$) and a mid threshold ($\delta \geq 0.1$).
	\begin{figure}[h!]
		\centering
		\subfloat{\includegraphics[width=0.5\linewidth]{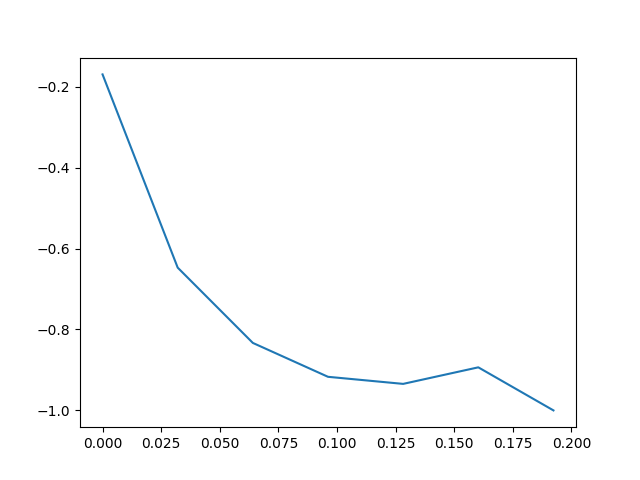}}
		\caption{\small Pearson Correlation Coefficient as a function of Threshold}
		\label{fig:t_v_corr}
	\end{figure}
	\subsubsection{Benefit to Visual Odometry:}
	We present a specific example to highlight the challenges faced by Visual Odometry algorithms when running on TIR camera images. The top sequence of \autoref{fig:svo-points} shows the points (Green) and Edgelets (Pink and Red) being tracked by SVO2.0 in the original dataset at frame ($t-2$, $t-1$ and $t$). Notice how the change in photometric error due to temporal variation lead to loss of feature tracking in SVO2.0 even though the algorithm was configured to correct for ``illumination gain and offset'' (terms used in SVO2.0 which is similar to temporal variation). The bottom sequence of \autoref{fig:svo-points} shows the same frames but after photometric calibration using the proposed method. Note that 1) more points are being tracked overall, and 2) tracking was successful in frame $t$.
	
	\begin{figure}[h!]
		\centering
		\subfloat{\includegraphics[width=0.32\linewidth]{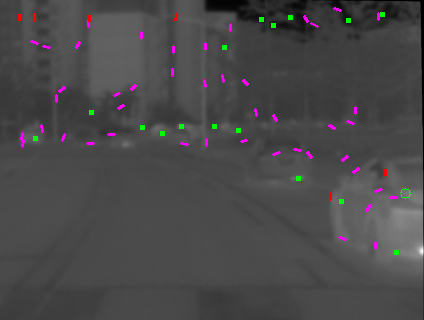}}\hfill
		\subfloat{\includegraphics[width=0.32\linewidth]{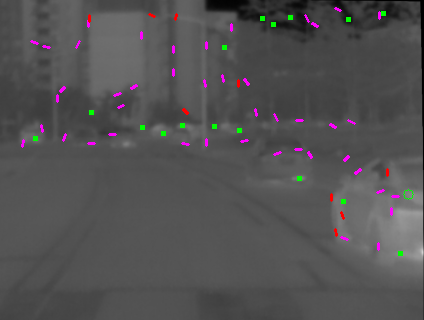}}\hfill
		\subfloat{\includegraphics[width=0.32\linewidth]{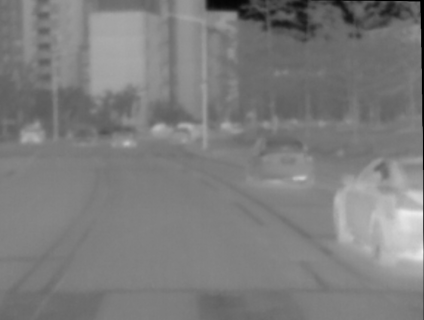}}\\
		\subfloat{\includegraphics[width=0.32\linewidth]{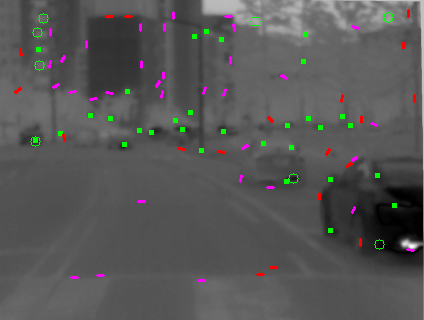}}\hfill
		\subfloat{\includegraphics[width=0.32\linewidth]{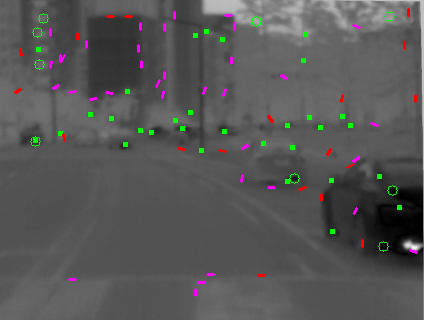}}\hfill
		\subfloat{\includegraphics[width=0.32\linewidth]{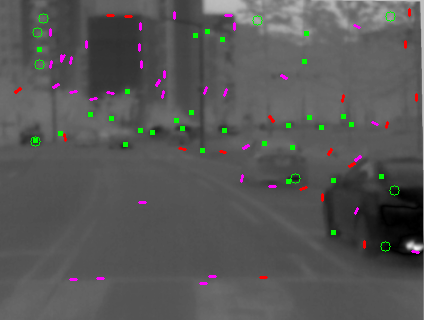}}
		\caption{\small Qualitative visualization of SVO2.0 tracking performance.\\ \textbf{Top:} Uncalibrated. \textbf{Bottom:} Calibrated. \textbf{Left to Right:} Frame at $t-2, t-1, t$} 
		\label{fig:svo-points}
	\end{figure}
	
	\subsubsection{With and Without Drift Adjustment:}
	\autoref{fig:PT_drift_gap} plots the temporal parameters ${}^1c_t$ (labelled as PT A) and ${}^1b_t$ (labelled as PT B) over the frames in Sequence AM05, before and after the proposed drift adjustments. Recall that the proposed method performs two adjustments in the estimated temporal parameters: 1) Gap adjustment: to maintain gap between ${}^1c_t$ and ${}^1b_t$ which in-effect maintains proper contrast in the image, and 2) Drift adjustment: to pull the parameteres towards their nominal values ($c=1$, $b=0$). As expected, we observe that gap adjustment is very important as otherwise the parameters might converge (${}^1c_t={}^1b_t$) or diverge. In the former case, during calibration the uncalibrated pixel intensity will be multiplied by $e^{{}^1a_t} = {}^1c_t-{}^1b_t = 0$, and thus will lead to total loss of information. Additionally, when the gap is low, the image will have low contrast and thus, feature initialization and tracking would suffer. Drift adjustment is performed to keep the range of image intensities consistent in the colormap output, which seems to improve tracking performance.
	\begin{figure}[h!]
		\centering
		\subfloat{\includegraphics[width=0.9\linewidth]{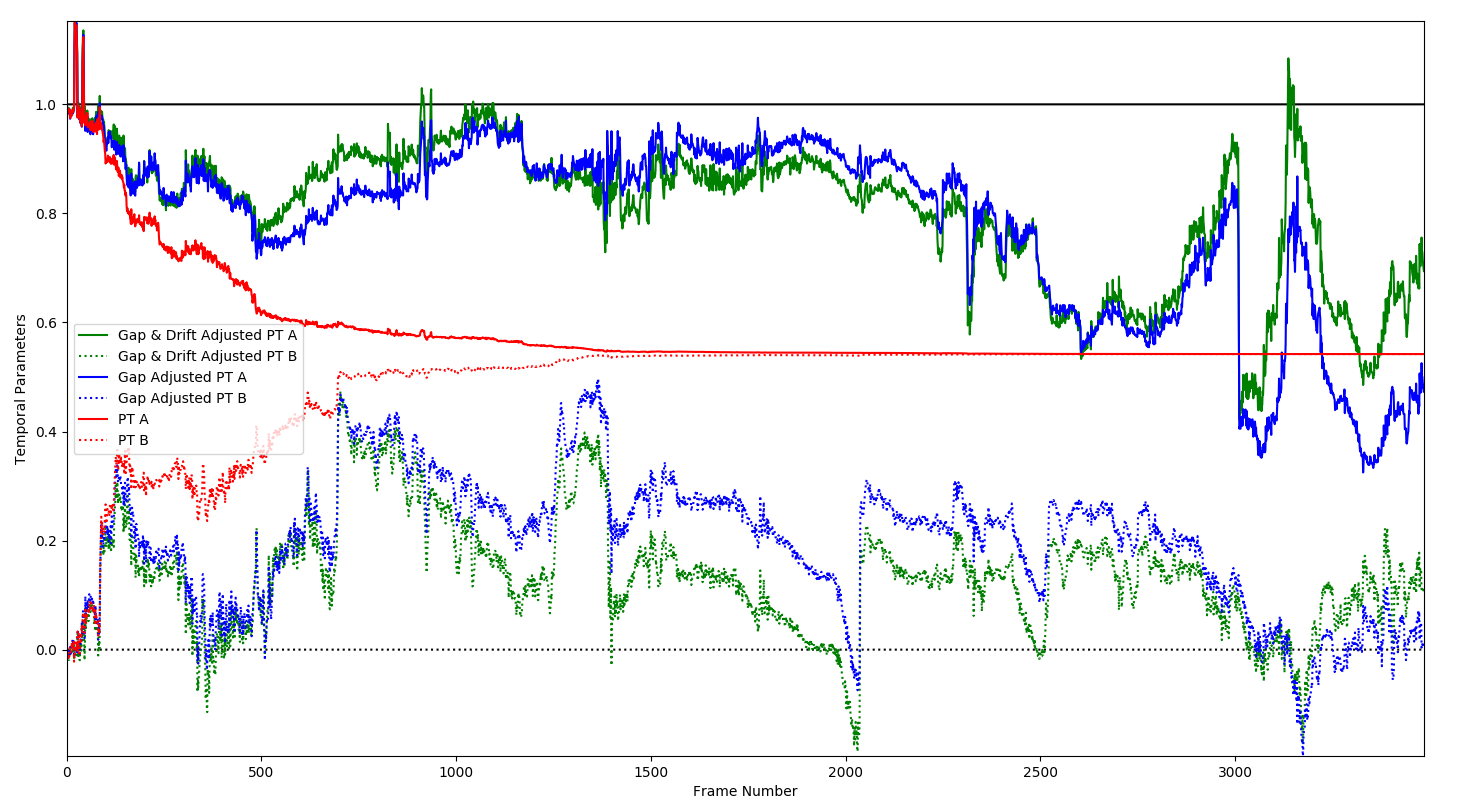}}
		\caption{\small Effect of Drift Adjustment and Gap Adjustment.}
		\label{fig:PT_drift_gap}
	\end{figure}
	
	\section{Appendix: Implementation Details}
	\subsubsection{Generating Feature Correspondences}
	We do not discuss in detail the algorithm to generate the pixel correspondences $C_t$, as the requirements of the proposed method is simply the correspondences between a pair of image frames. To that extent, there exists various algorithms to find these correspondences. Even if these algorithms suffer due to photometric errors, RANSAC method employed by the proposed approach makes it robust to outliers, and connected components based estimation of spatial parameters ensure correct estimation once a lot of such frame-pair-wise pixel correspondences are found over a lot of consecutive frames. However, due to very low contrast images of TIR cameras, we observed that feature tracker as used in Direct Sparse Odometry algorithms delivers robust performance.
	
	\subsubsection{Gaussian Process Regression on Spatial Parameters}
	\autoref{fig:PS_GP} visualizes the estimated spatial parameteres $\mathcal{P}_s$ (\textbf{Left}), once in ``jet'' colormap (\textbf{Top}) to make the changes more more distinct and once in ``grayscale'' (\textbf{Bottom}) to give a sense of what is actually applied to the image during calibration. The spatial parameters after Gaussian Process Regression using Squared Exponential Kernel is shown on the \textbf{Right}. Recall that the estimated spatial parameteres are subtracted from the image during calibration. Thus, in the grayscale version, regions that appear more white signifies a larger value for subtraction. For eg.\, \autoref{fig:PS_GP} shows the parameters for MAV\_B dataset where we observed that the top-right corner is over-exposed and the bottom regions are under-exposed.
	\begin{figure}[h!]
		\centering
		\subfloat{\includegraphics[width=0.8\linewidth]{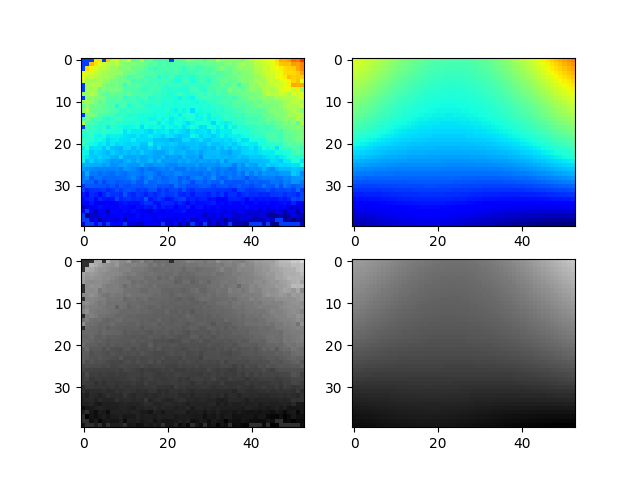}}
		\caption{\small Spatial parameteres for MAV\_B dataset.}
		\label{fig:PS_GP}
	\end{figure}
